# Supplementary material for: GFreeDet: Exploiting Gaussian Splatting and Foundation Models for Model-free Unseen Object Detection in the BOP Challenge 2024
Source: arXiv:2412.01552 source file (2025-04-23)
Supplement: Supplementary file 1 [file 12_appendix.tex]

\section{Appendix Section}
\label{sec:appendix_section}
Supplementary material goes here.
